# Supplementary material for: VILA: On Pre-training for Visual Language Models
Source: arXiv:2312.07533 source file (2024-05-16)
Supplement: Supplementary file 1 [file supp.tex]

% \documentclass[10pt,twocolumn,letterpaper]{article}

% %%%%%%%%% PAPER TYPE  - PLEASE UPDATE FOR FINAL VERSION
% % \usepackage{cvpr}              % To produce the CAMERA-READY version
% \usepackage[review]{cvpr}      % To produce the REVIEW version
% % \usepackage[pagenumbers]{cvpr} % To force page numbers, e.g. for an arXiv version

% \input{package}
% \input{macro}

% % \input{preamble}

% %%%%%%%%% PAPER ID  - PLEASE UPDATE
% \def\paperID{5738}
% \def\confName{CVPR}
% \def\confYear{2024}

% \begin{document}

% %%%%%%%%% TITLE
% \title{Supplementary Material \\ \methodshort: On Pre-training for Visual Language Models}

% \author{TODO
% }

% \maketitle

% % \thispagestyle{empty}
% % \pagestyle{empty}

% \appendix
 
%  \input{text/appendix} 

% \clearpage
% {\small
% \bibliographystyle{ieeenat_fullname}
% \bibliography{main}
% }

% % \clearpage

% \end{document}
